# Supplementary material for: Reliability and Robustness analysis of Machine Learning based Phishing URL Detectors
Source: arXiv:2005.08454 source file (2022-11-24)
Supplement: Supplementary file 1 [file Appendix.tex]

\begin{table*}[!tb]
  \caption{Hyper-parameter selected for traditional ML Models (T-MLPU)}
  \label{hyper}
\begin{small}
\resizebox{\textwidth}{!}{ \begin{tabular}{c|c|c|c|c|c|c|c}
\hline
\textbf{Classifiers}&\textbf{Parameters}&\textbf{Basic} &\textbf{BoW}&\textbf{Bigram} &\textbf{Char} &\textbf{BoW of}&\textbf{Basic Lexical}\\
&&\textbf{Lexical}&&&\textbf{n-gram}& \textbf{URL parts}&+\textbf{External}\\
\hline
\multirow{3}{*}{\textbf{RF}}&criterion&entropy&gini&gini&gini&entropy&entropy\\
\cline{2-8}
&max\_depth&194&4&18&44&24&79\\
\cline{2-8}
&n\_estimators&64&70&38&26&99&57\\
\hline
\multirow{4}{*}{\textbf{DT}}&criterion&entropy&gini&gini&gini&entropy&entropy\\
\cline{2-8}
&max\_depth&110&19&24&57&39&120\\
\cline{2-8}
&normalize&0&1&0&0&1&0\\
\cline{2-8}
&scale&0&0&0&0&0&0\\
\hline
\multirow{2}{*}{\textbf{SVM}}&C&0.09&15.24&7.49&2.02&8&0.85\\
\cline{2-8}
&scale&1&0&0&0&0&1\\
\hline
\multirow{6}{*}{\textbf{LR}}&C&1.57&2.87&2.58&1.72&2.64&2.92\\
\cline{2-8}
&fit\-intercept&0&0&0&0&0&0\\
\cline{2-8}
&max\_iter&66&5&199&205&222&873\\
\cline{2-8}
&normalize&0&0&0&0&0&0\\
\cline{2-8}
&scale&0&0&0&0&0&1\\
\cline{2-8}
&solver&newton-cg&newton-cg&newton-cg&newton-cg&newton-cg&liblinear\\
\cline{2-8}
&tol&6.42E-05&9.77E-05&9.51E-05&3.10E-05&8.58E-05&9.49E-05\\
\cline{2-8}
&warm\_start&1&0&0&1&1&1\\
\hline
\multirow{3}{*}{\textbf{KNN}}&n\_neighbors&0&0&0&1&4&39\\
\cline{2-8}
&normalize&1&1&0&1&1&0\\
\cline{2-8}
&scale&1&0&0&0&0&1\\
\hline
\multirow{2}{*}{\textbf{XGB}}&max\_depth&92&99&147&150&100&51\\
\cline{2-8}
&tree\_method&exact&exact&exact&hist&exact&approx\\
\hline
\multirow{3}{*}{\textbf{LGBM}}&learning\_rate&2&1&3&1&2&4\\
\cline{2-8}
&num\_leave&296&179&193&289&298&280\\
\hline

\end{tabular}}
\end{small}
\end{table*}.
